# Supplementary material for: 3D Spatial Pattern Matching
Source: arXiv:2606.26465 source file (2026-06-25)
Supplement: Supplementary file 1 [file 70_Appendix.tex]

% ```latex
% \begin{lstlisting}[
% caption={Cypher query used to extract geometric and semantic building attributes together with facade opening information from the property knowledge graph.},
% label={lst:cypher_query}
% ]
% MATCH (b:Building)
% OPTIONAL MATCH (b)-[:HAS_ROOF_MATERIAL]->(rm:RoofMaterial)
% OPTIONAL MATCH (b)-[:HAS_ROOF_TYPE]->(rt:RoofType)
% OPTIONAL MATCH (b)-[:HAS_FACADE_OPENING]->(o:Opening)

% WITH b, rm, rt, collect(o) AS openings

% UNWIND CASE
%     WHEN size(openings) = 0 THEN [null]
%     ELSE openings
% END AS op

% RETURN
%     b.id AS gml_id,
%     rm.name AS material,
%     rt.code AS roofType,
%     toFloat(b.measured_height) AS measured_height,
%     b.storeys_above_ground AS storeysAboveGround,

%     toFloat(b.bbox_max_x) AS upperCorner_x,
%     toFloat(b.bbox_max_y) AS upperCorner_y,
%     toFloat(coalesce(b.bbox_max_z, b.ground_z, 0.0))
%         + toFloat(coalesce(b.measured_height, 0))
%         AS upperCorner_z,

%     toFloat(b.bbox_min_x) AS lowerCorner_x,
%     toFloat(b.bbox_min_y) AS lowerCorner_y,
%     toFloat(coalesce(b.ground_z, b.bbox_min_z, 0.0))
%         AS lowerCorner_z,

%     op.type AS opening_type,

%     toFloat(b.bbox_min_x)
%         + toFloat(op.u0)
%         * (toFloat(b.bbox_max_x) - toFloat(b.bbox_min_x))
%         AS opening_x1_utm,

%     toFloat(b.bbox_min_x)
%         + toFloat(op.u1)
%         * (toFloat(b.bbox_max_x) - toFloat(b.bbox_min_x))
%         AS opening_x2_utm,

%     toFloat(coalesce(b.ground_z, 0.0))
%         + toFloat(op.v0) * toFloat(b.measured_height)
%         AS opening_y1_utm,

%     toFloat(coalesce(b.ground_z, 0.0))
%         + toFloat(op.v1) * toFloat(b.measured_height)
%         AS opening_y2_utm,

%     toFloat(
%         coalesce(
%             b.center_y,
%             (b.bbox_min_y + b.bbox_max_y) / 2.0
%         )
%     ) AS opening_z_utm

% ORDER BY gml_id
% \end{lstlisting}
% ```
